# Supplementary material for: Efficient generation of many-body entangled states by multilevel oscillations
Source: arXiv:1907.13310 source file (2019-07-31)
Supplement: Supplementary file 1 [file supp.pdf]

# Supplemental Material: Efficient generation of many-body entangled states by multi-level oscillations

Peng Xu,[1] Su Yi,[2,3] and Wenxian Zhang[1,*]

[1]*School of Physics and Technology, Wuhan University, Wuhan, Hubei 430072, China*
[2]*CAS Key Laboratory of Theoretical Physics, Institute of Theoretical Physics, Chinese Academy of Sciences, P.O. Box 2735, Beijing 100190, China*
[3]*School of Physical Sciences & CAS Center for Excellence in Topological Quantum Computation, University of Chinese Academy of Sciences, Beijing 100049, China*

(Dated: June 17, 2019)

## I. MULTI-LEVEL OSCILLATION FOR A HARMONIC OSCILLATOR

As mentioned in the main text, the Hamiltonian of an oscillator with a mass $M$ in an extra linear potential reads [1],

$$H_o = \frac{P^2}{2M} + \frac{1}{2}M\omega^2 x^2 + V(x), \tag{1}$$

where $P$ is the momentum, $x$ the position, $\omega$ the trapping angular frequency, and $V(x) = Fx$ with $F$ the force for the oscillator. The eigenstates of this system are $\psi_n(x+x_0)$ for $H_o(F=F_0)$, $\psi_n(x)$ for $H_o(F=0)$ and $\psi_n(x-x_0)$ for $H_o(F=-F_0)$, respectively. The ground states are respectively $\psi_0(x+x_c) = \pi^{-1/4}\alpha^{1/2}e^{-\alpha^2(x+x_c)^2/2}$ with $x_c = \pm x_0, 0$, $\alpha = \sqrt{M\omega/\hbar}$, and $x_0 = F/(M\omega^2)$.

We expand the initial state $\psi_0(x+x_0)$ and the target state $\psi_0(x-x_0)$ in the space spanned by the eigenstates of the Hamiltonian $H_o(F=0)$

$$\psi_0(x+x_0) = \sum_{n=0}^{\infty} C_n\psi_n(x),$$
$$\psi_0(x-x_0) = \sum_{n=0}^{\infty} C'_n\psi_n(x). \tag{2}$$

The coefficients $C_n$ and $C'_n$ are calculated as

$$C_n = \frac{(-1)^n}{\sqrt{2^n n!}}\zeta_0^n e^{-\zeta_0^2/4},$$
$$C'_n = \frac{1}{\sqrt{2^n n!}}\zeta_0^n e^{-\zeta_0^2/4}, \tag{3}$$

where $\zeta_0 = \alpha x_0$. The initial state $\psi_0(x+x_0)$ oscillates under the Hamiltonian $H_o(F=0)$. It is easy to calculate the probability of the oscillator on the $n$th instantaneous eigenstate $|C_n|^2$. Obviously, this probability is time independent. While in the final Hamiltonian's eigenenergy basis, the probability of the ground state is

$$|\langle\psi_0(x-x_0)|e^{-iH_o t}|\psi_0(x+x_0)\rangle|^2 = |\sum_{n=0}^{\infty} C_n C'_n e^{-in\omega t}|^2.$$

As shown by the above equation, the probability of the oscillator on the ground state $\psi_0(x-x_0)$ oscillates. In particular, when $t = \pi/\omega$, the probability equals 100%. Obviously, this multilevel oscillation is an analogy to the two-level Rabi oscillation. Through this single multilevel oscillation, the oscillator reaches the same target state as the result with an adiabatic process but in a much shorter period. More importantly, this multilevel oscillation process is much easier to implement in experiments than the adiabatic one.

## II. DERIVATION OF THE EFFECTIVE HAMILTONIAN

The system we consider is an antiferromagnetic spin-1 Bose-Einstein condensate in an external magnetic field, which has been realized with $^{23}$Na atoms in an optical trap [2, 3]. The Hamiltonian of this system can be divided into two parts

$$H = H_0 + H_i\ , \tag{4}$$

where the non-interacting Hamiltonian $H_0$ and the interaction Hamiltonian $H_i$ take respectively the following forms [4–6]

$$H_0 = \int d\boldsymbol{r}\hat{\Psi}^\dagger_m(\boldsymbol{r})\left[\left(-\frac{\hbar^2\nabla^2}{2M} + U(\boldsymbol{r})\right)\delta_{mn} - p(f_z)_{mn} + q(f_z^2)_{mn}\right]\hat{\Psi}_n(\boldsymbol{r}),$$
$$H_i = \frac{c_0}{2}\int d\boldsymbol{r}\hat{\Psi}^\dagger_m(\boldsymbol{r})\hat{\Psi}^\dagger_n(\boldsymbol{r})\hat{\Psi}_m(\boldsymbol{r})\hat{\Psi}_n(\boldsymbol{r}) + \frac{c_2}{2}\int d\boldsymbol{r}\hat{\Psi}^\dagger_m(\boldsymbol{r})\hat{\Psi}^\dagger_{m'}(\boldsymbol{r})\boldsymbol{f}_{mn}\cdot\boldsymbol{f}_{m'n'}\hat{\Psi}_n(\boldsymbol{r})\hat{\Psi}_{n'}(\boldsymbol{r}),$$

where $M$ is the mass of the atom, $\hat{\Psi}_m$ the field annihilation operator for spin component $m = \pm1, 0$. $\boldsymbol{f} = (f_x, f_y, f_z)$ with $f_{x,y,z}$ being spin-1 matrices. The linear Zeeman coefficient $p = -g\mu_B B$, where $g$ is the Landé g factor, $\mu_B$ the Bohr magneton, and $B$ the external magnetic field. The quadratic Zeeman coefficient $q = q_{_{MW}} + (g\mu_B B)^2/\Delta E_{hf} \approx q_{_{MW}} + B^2\times$ 277 Hz/G$^2$ for $^{23}$Na, where $\Delta E_{hf}$ is the hyperfine energy splitting and $q_{_{MW}}$ is the level shift induced by a microwave field [7–9]. The collision interaction parameters are $c_0 = 4\pi\hbar^2(a_0+2a_2)/3M$ and $c_2 = 4\pi\hbar^2(a_2-a_0)/3M$

* Corresponding email: wxzhang@whu.edu.cn

with $a_{0(2)}$ being the $s$-wave scattering length of two spin-1 atoms in the combined symmetric channel of total spin 0(2). We have $c_2 > 0$ for $^{23}$Na, which corresponds to antiferromagnetic spin interaction.

For a typical spinor condensate such as $^{23}$Na, the spin-independent interaction dominates over the spin-dependent interaction since $c_0 \gg |c_2|$. In this case, the single mode approximation is good to describe the ground state in a trap. Under this single mode approximation [5, 10, 11], $\hat{\Psi}_m(\boldsymbol{r}) \simeq \phi(\boldsymbol{r})\hat{a}_m$ with $\phi(\boldsymbol{r})$ being a spin-independent spatial mode function and $\hat{a}_m$ the annihilation operator of spin component $m$. We assume the spinor condensate has a fixed total particle number $N$ and neglect the constant terms in the Hamiltonian. The final spin-dependent Hamiltonian we consider is remarkably simplified as

$$H = c_2' \frac{\boldsymbol{L}^2}{N} + \sum_{m=\pm1,0} (qm^2 - pm) a_m^\dagger a_m, \tag{5}$$

where $c_2' = c_2 N \int d\boldsymbol{r}|\phi(\boldsymbol{r})|^4/2$ and $\boldsymbol{L} \equiv \sum_{mn} \hat{a}_m^\dagger \boldsymbol{f}_{mn} \hat{a}_n$.

The linear Zeeman term $\sum_{m=\pm1,0} pma_m^\dagger a_m = pL_z$ usually dominates in the Hamiltonian $H$. However, this term commutes with the whole Hamiltonian and can be neglected. The effective spin Hamiltonian becomes [12, 13]

$$H_e = c_2' \frac{\boldsymbol{L}^2}{N} - q a_0^\dagger a_0. \tag{6}$$

In $^{23}$Na spin-1 condensate experiment, a typical value of $c_2'$ can be estimated in a spherical trap with frequencies $(\omega_x, \omega_y, \omega_z) = 2\pi \times (600, 600, 600)$ Hz, and its value is approximately 25 Hz for $N = 1,000$ by assuming a Gaussian ansatz.

## III. GROUND STATE OF HAMILTONIAN $H_e$

In the limit $q \to \infty$, the term $-qa_0^\dagger a_0$ dominates in the Hamiltonian $H_e$. The ground state is given by an eigenstate of $a_0^\dagger a_0$ with the maximum eigenvalue $N_0 = N$ (polar state). While, in the opposite direction $q \to -\infty$, the ground state is given by an eigenstate of $a_0^\dagger a_0$ with the minimum eigenvalue $N_0 = 0$ for total even atom number (twin-Fock state), and $N_0 = 1$ for total odd atom number.

At the point $q = 0$, the many-body singlet state $|l = 0, m_l = 0\rangle$ and $|l = 1, m_l = 0\rangle$ are the ground states of $H_e$ for even and odd atom number, respectively. Using the Fock basis $|N_1, N_0, N_{-1}\rangle$, defined by the number operators $\hat{N}_m \equiv \hat{a}_m^\dagger \hat{a}_m$ for three spin components (i.e. $\hat{N}_m|N_1, N_0, N_{-1}\rangle = N_m|N_1, N_0, N_{-1}\rangle$), the singlet state $|l = 0, m_l = 0\rangle$ has the form [5]

$$|l = 0, m_l = 0\rangle = \sum_{k=0}^{N/2} A_k |k, N-2k, k\rangle, \tag{7}$$

where the amplitudes $A_k$ obey the recursion relation

$$A_k = -A_{k-1}\sqrt{\frac{N-2k+2}{N-2k+1}}\,. \tag{8}$$

In addition, the state $|l = 1, m_l = 0\rangle$ has the form

$$|l = 1, m_l = 0\rangle = \sum_{k=0}^{(N-1)/2} A_k |k, N-2k, k\rangle, \tag{9}$$

and the amplitudes $A_k$ obey another recursion relation

$$A_k = -A_{k-1}\sqrt{\frac{N-2k+1}{N-2k+2}}\,. \tag{10}$$

## IV. LINK BETWEEN THE SPIN-1 BEC AND THE HARMONIC OSCILLATOR

The effective Hamiltonian $H_e$ in Eq. (6) can also be described in the eigenenergy basis $|l\rangle \equiv |N, l, m_l = 0\rangle$ for $q = 0$. The spin-exchange term becomes diagonal, while the operator $a_0^\dagger a_0$ becomes off-diagonal and couples the states $l$ and $l \pm 2$. The action of the operator $a_0^\dagger a_0$ is [14]

$$a_0^\dagger a_0|l\rangle = \sqrt{A_l B_{l+2}}|l+2\rangle + \sqrt{A_{l-2}B_l}|l-2\rangle + [A_l + B_l]|l\rangle,$$

where

$$A_l = \frac{(l+1)^2(N-l)}{(2l+1)(2l+3)},$$
$$B_l = \frac{l^2(N+l+1)}{(2l+1)(2l-1)}.$$

The resulting Schrödinger equation now reads

$$i\dot{\beta}_l = h_{l,l+2}\beta_{l+2} + h_{l,l-2}\beta_{l-2} + h_{l,l}\beta_l, \tag{11}$$

where

$$h_{l,l+2} = -q\sqrt{A_l B_{l-2}},$$
$$h_{l,l-2} = -q\sqrt{A_{l-2} B_l},$$
$$h_{l,l} = \frac{c_2'}{N} l(l+1) - q[A_l + B_l].$$

Similarly, the equation of motion for the harmonic oscillator in the eigenenergy basis $|n\rangle$ for $F = 0$ is

$$i\dot{C}_n = g_{n,n+1}C_{n+1} + g_{n,n-1}C_{n-1} + g_{n,n}C_n, \tag{12}$$

where $g_{n,n+1} = F\sqrt{(n+1)/2M\omega}$, $g_{n,n-1} = F\sqrt{n/2M\omega}$, and $g_{n,n} = E_n$ with $E_n$ the eigenenergy of the simple harmonic oscillator.

Obviously, these two systems have the same chain-form Schrödinger equations shown in Eq. (11) and Eq. (12) except for different coefficients [15]. Furthermore, according to Refs. [16–18], when there is a small change of the quadratic Zeeman splitting $q$, the oscillations of the antiferromagnetic spin-1 BEC exhibit the same feature as the harmonic oscillator. As shown in Fig. 1, for the harmonic oscillator, all levels share the same frequency and

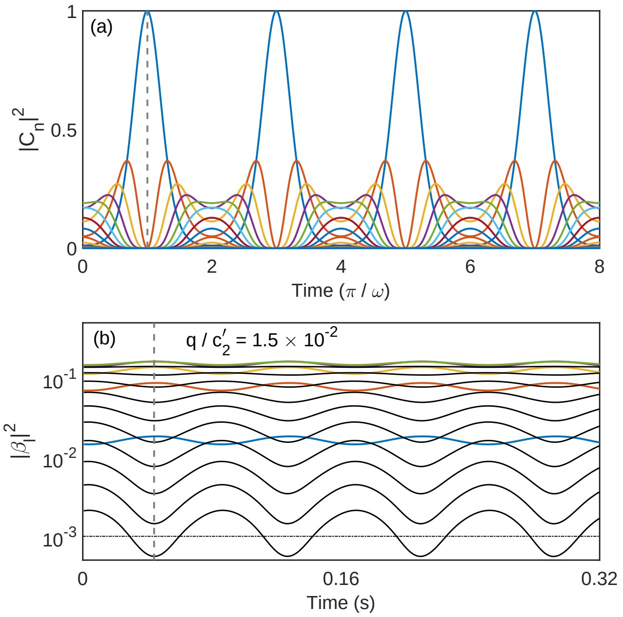


FIG. 1. (Color online.) (a) The multilevel oscillation for a harmonic oscillator in the eigenenergy basis of the Hamiltonian Eq. (1) with $F = -F_0$. The initial state is the ground state of the Hamiltonian with $F = F_0$. The dynamics is under the Hamiltonian with $F = 0$. After a half-period $\pi/\omega$ (vertical grey dashed line), the oscillator reaches the ground state of the Hamiltonian with $F = -F_0$. (b) The multilevel oscillation of an antiferromagnetic spin-1 BEC in the eigenenergy basis of the Hamiltonian Eq. (6) with $q = 0$. The initial state is the ground state of the Hamiltonian with $q/c_2' = 0.0315$ ($q = 0.788$ Hz with $c_2' = 25$ Hz). The dynamics is under the Hamiltonian with $q/c_2' = 1.5 \times 10^{-2}$. After a half-period (vertical grey dashed line), the probabilities of higher levels (black solid lines) oscillate to small values, while the probabilities of lower levels (color solid lines) oscillate to bigger values.

the probabilities of higher levels are totally transferred to the ground state of Hamiltonian with $F = -F_0$ after a half-period $\pi/\omega$. For the spin-1 BEC, all levels almost share the same frequency when there is a small change of $q$ (from $q/c_2' = 3.15 \times 10^{-2}$ to $q/c_2' = 1.5 \times 10^{-2}$). Such a harmonic oscillation shown in Fig. 1(b) confirms the result of Ref. [16–18] that there locally exists a harmonic oscillator in the antiferromagnetic spin-1 BEC. This inspires us that the multilevel oscillation may be employed in the antiferromagnetic spin-1 BEC to stepwise eliminate the higher level probabilities and eventually reach the ground state of the Hamiltonian with $q = 0$. In the next section of the SM, we numerically find an optimized range of $q$, which maximizes the total probabilities of the lower levels. We also explore regions slightly beyond the harmonic region with bigger changes of $q$.

## V. OPTIMIZATION OF QUADRATIC ZEEMAN SPLITTING $q$

To better understand the multilevel oscillations, we describe the process in the eigenenergy basis for $q = 0$. Any state $|\psi\rangle$ is expanded as $\sum_{l=0}^{N} \beta_l |l\rangle$ ($l$ is an even integer), where $|0\rangle$, $|2\rangle$, $|4\rangle$, $\cdots$, $|N\rangle$ are the eigenstates of the Hamiltonian $H_e$ with $q = 0$. We define an eigenenergy level as occupied if the probability $|\beta_l|^2 > 0.1\%$. For a given state at a time, we calculate $|\beta_l|^2$ and count the number of occupied levels $K$. At the beginning of the first multilevel oscillation, we find the number of occupied levels for $|\psi(t = 0.9 \text{ s})\rangle$ is $K = 15$ for $N = 1,000$. The goal of the multilevel oscillations is to reduce the number of occupied levels $K$ from 15 to 1, i.e., to the singlet state. In general, the probability $|\beta_l|^2$ for each multilevel oscillation is a function of the quadratic Zeeman splitting $q$ and the evolution time $t$. For a given constant $q$, we evolve the system and monitor the number of occupied levels $K$ till $K$ reaches its first local minimum $K(q)$. For different $q$, we again minimize $K(q)$ in a certain range where the spin exchange term and the quadratic Zeeman term are comparable, i.e., $q\langle a_0^\dagger a_0\rangle \sim c_2'\langle \boldsymbol{L}^2/N\rangle$ with the average over the highest occupied state.

We present in detail the procedure to optimize the quadratic Zeeman splitting $q$ for a total atom number $N = 1,000$. For the first multilevel oscillation, we estimate the spin exchange term by averaging over the fifteenth $|28\rangle$ eigenstate, $\sim \langle 28|\boldsymbol{L}^2|28\rangle/N^2 = 8.12 \times 10^{-4}$, because there are 15 occupied levels right after the adiabatic evolution. As an example, we randomly choose $q/c_2' = 9.2 \times 10^{-4}$ and the spin-1 BEC evolves under this Hamiltonian. As shown in Fig. 2(a), despite that the dynamics goes slightly beyond the harmonic region, the number of occupied levels $K$ constantly decreases with time and a platform appears where $K$ is minimal, as shown in Fig. 2(d). We denote this platform as the minimal number of occupied levels $K(q)$, which is marked as a diamond in Fig. 3(a). Similarly, two other random values of $q$ are chosen and the corresponding numerical results are shown in Figs. 2(b, e) and Figs. 2(c, f). We also find the minimal number of occupied levels $K(q/c_2' = 1.2 \times 10^{-3}) = 4$ and $K(q/c_2' = 2.2 \times 10^{-3}) = 6$ which are marked respectively as a cross and a star in Fig. 3(a).

By numerically sweeping $q/c_2'$ in this vicinity $\sim \langle 28|\boldsymbol{L}^2|28\rangle/N^2 = 8.12 \times 10^{-4}$ for the first multilevel oscillation, the minimal number of occupied levels $K(q)$ as a function of $q$ is shown in Fig. 3(a). We find there exists a range of $q$, where $K(q)$ always equal to 4 and $K(q)$ becomes larger otherwise. Our goal is to reduce $K(q)$ to a smallest value during each multilevel oscillation. We then take randomly the value $q/c_2' = 1.2 \times 10^{-3}$ as an example and the corresponding dynamics during $[0.9, 1.05]$

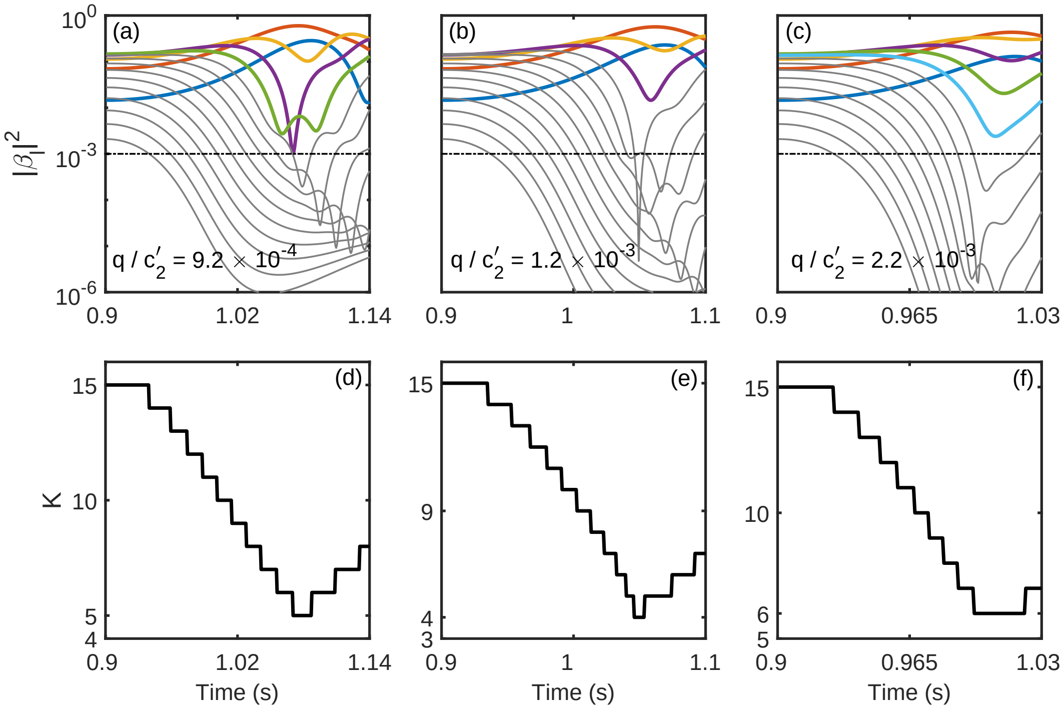


FIG. 2. (Color online.) Typical dynamics of the first multilevel oscillation for (a, d) $q/c_2' = 9.2 \times 10^{-4}$, (b, e) $q/c_2' = 1.2 \times 10^{-3}$, (c, f) $q/c_2' = 2.2 \times 10^{-3}$. (d-f) Time dependence of the number of occupied levels $K$. The total atom number is $N = 1,000$.

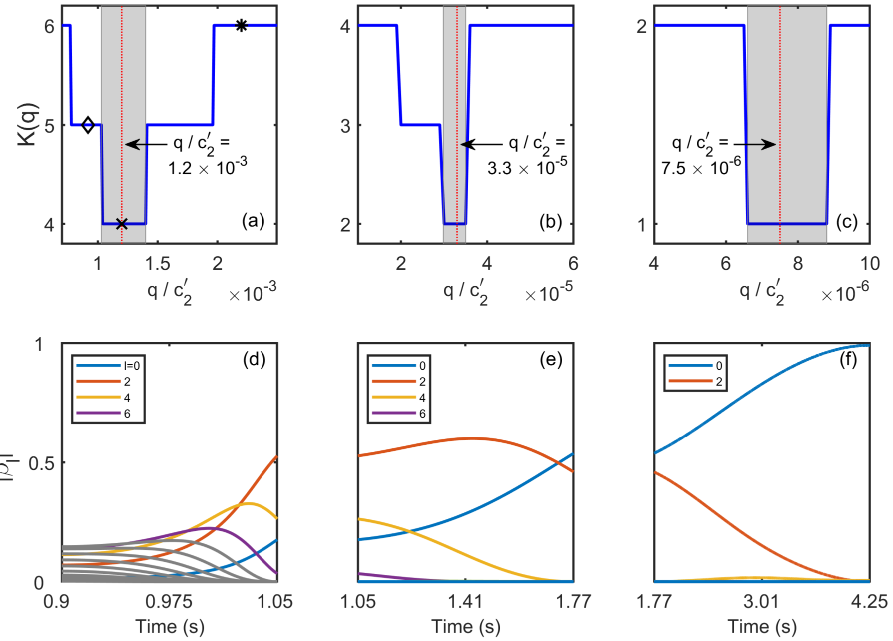


FIG. 3. (Color online.) The minimal number of occupied levels $K(q)$ for different $q/c_2'$ for (a) the first, (b) the second, and (c) the third multilevel oscillation. Typical evolution for (d) $q/c_2' = 1.2\times10^{-3}$ in the first multilevel oscillation, (e) $q/c_2' = 3.3\times10^{-5}$ in the second and (f) $q/c_2' = 7.5 \times 10^{-6}$ in the third. The total atom number is $N = 1,000$.

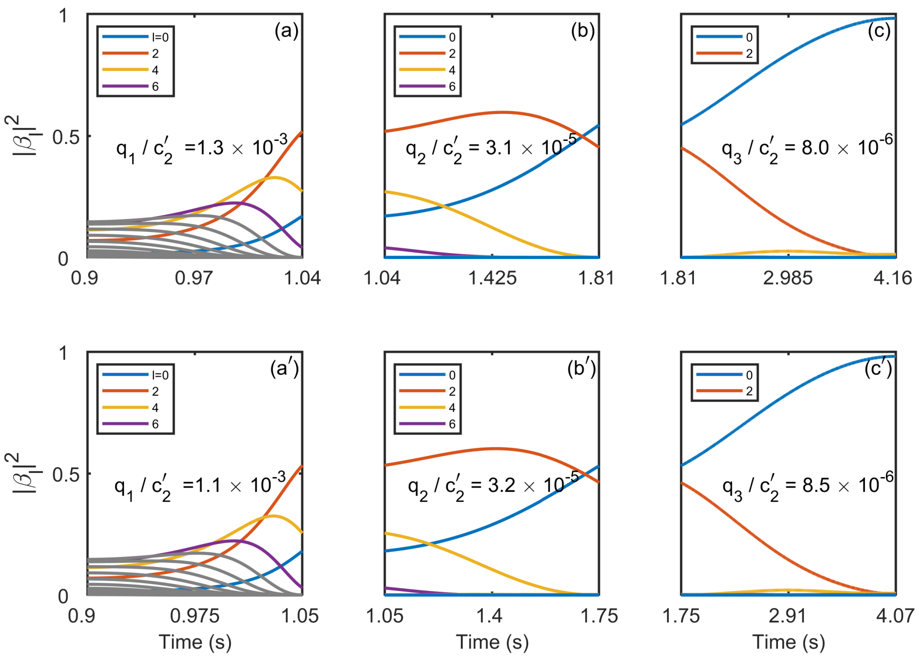


FIG. 4. (Color online.) Typical evolutions for two different sets of $q$, with $\{q_1/c_2' = 1.3 \times 10^{-3}$, $q_2/c_2' = 3.1 \times 10^{-5}$, $q_3/c_2' = 8.0 \times 10^{-6}.\}$ in (a-c); with $\{q_1/c_2' = 1.1 \times 10^{-3}$, $q_2/c_2' = 3.2 \times 10^{-5}$, $q_3/c_2' = 8.5 \times 10^{-6}.\}$ in (a'-c'). The total atom number is $N = 1,000$.

s is shown in Fig. 3(d). The stop time is also randomly set $t = 1.05$ but guarantees $K = 4$. Clearly, the high energy states oscillate out as shown in Fig. 2(b, e).

For the second multilevel oscillation, since there are just 4 occupied levels, we sweep $q/c_2'$ in the vicinity of $\langle 6|\boldsymbol{L}^2|6\rangle/N^2 = 4.2 \times 10^{-5}$. It is easy to check that the $q$ term does not recouple the eliminated higher levels during the first multilevel oscillation, because of the large detuning between any pair of the nearest higher levels. The results for the second multilevel oscillation are shown in Fig. 3(b). We then take $q/c_2' = 3.3 \times 10^{-5}$ and show the corresponding dynamics during $[1.05, 1.77]$ s in Fig. 3(e). The number of occupied levels is reduced to 2. For the third multilevel oscillation, we use the Rabi oscillation for the two levels with $q/c_2' = 7.5 \times 10^{-6}$ which is in the vicinity of $\langle 2|\boldsymbol{L}^2|2\rangle/N^2 = 6 \times 10^{-6}$ during $[1.77, 4.25]$ s. We eventually obtain a singlet state with a fidelity higher than 99%. Although we present one set of the control parameter $q$, it is easy to find other sets of $\{q_1, q_2, q_3\}$ under the condition that $K(q_1) = 4$ in the first multilevel oscillation, $K(q_2) = 2$ in the second, and $K(q_3) = 1$ in the third. In Fig. 4, we show two different sets of $q$ as examples in multilevel oscillations to efficiently generate the singlet state.

As elegant as above procedure of optimizing the quadratic Zeeman splitting $q$ based on the number of occupied levels, however, in real experiment, it is impossible to monitor the number of occupied levels during the multilevel oscillation process. Instead, we choose the

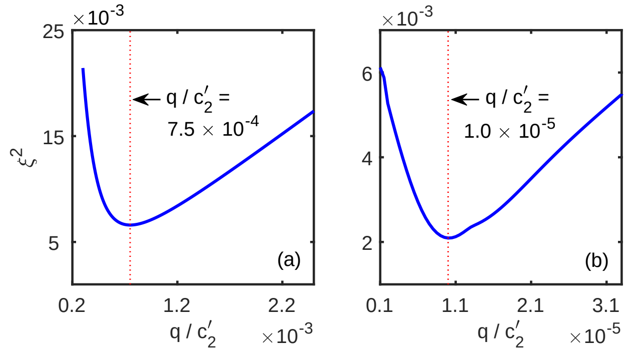


FIG. 5. (Color online.) The generalized squeezing parameter $\xi^2$ for different $q/c_2'$ for (a) the first and (b) the second multilevel oscillation. The optimal $q$s for the two multilevel oscillations are marked by red dotted lines.

generalized squeezing parameter $\xi^2$. Under the similar optimizing process as shown in Fig. 3, we numerically obtain $\xi^2(q)$ as a function of $q/c_2'$ as shown in Fig. 5. By considering the real experimental condition about the quadratic Zeeman splitting, which is limited by a lower bound due to the stray magnetic fields ($\delta B_z \sim 0.1$ mG), we need just two multilevel oscillation processes, because $q = 1.0 \times 10^{-5} c_2'$ equivalent to a bias field $B_z = 0.95$ mG with $c_2' = 25$ Hz and $B_z \gg \delta B_z$. The corresponding dynamics about $\xi^2$ for $q/c_2' = 1.0 \times 10^{-5}$ after $q/c_2' = 7.5 \times 10^{-4}$ are shown in Fig. 6(a).

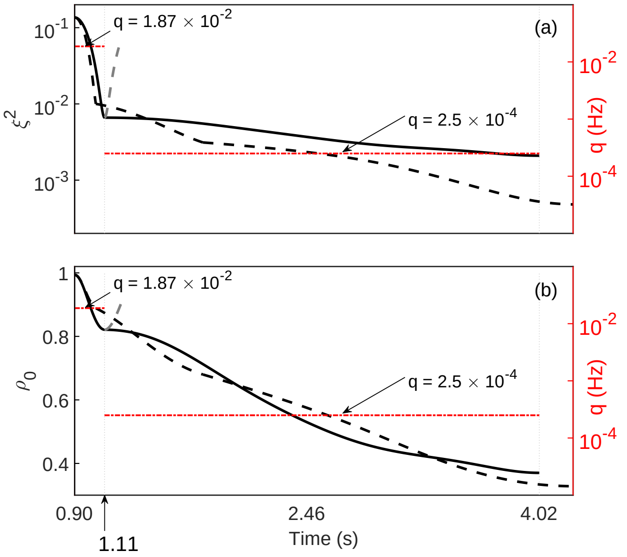


FIG. 6. (Color online.) Typical dynamics about (a) $\xi^2$ and (b) $\rho_0$ for $q/c_2' = 1.0 \times 10^{-5}$ after $q/c_2' = 7.5 \times 10^{-4}$ ($c_2' = 25$ Hz). The total atom number is $N = 1,000$. The dashed lines are the optimization results with the same parameters as in Fig. 3.

In each multilevel oscillation after we quench the quadratic Zeeman splitting, the total energy of system is conserved. Such a conservation results in that the fractional population $\rho_0(t) = \langle N_0 \rangle / N$ and $\xi^2(t) \propto \langle \boldsymbol{L}^2 \rangle$ simultaneously reach their respective stationary point in the multilevel oscillation processes, where $\langle \boldsymbol{L} \rangle = 0$. Therefore, optimizing $\xi^2$ is equivalent to optimizing $\rho_0$. We may utilize such an equivalence to monitor the second multilevel oscillation, i.e, monitoring the evolution of $\rho_0$ instead of $\xi^2$ (too small to detect experimentally). Indeed, this replacement works well, as shown in the numerical simulation presented in Fig. 6. Although in the second multilevel oscillation, the squeezing parameter $\xi^2$ does not decrease as drastically as the first multilevel oscillation, the fractional population $\rho_0$ decreases significantly and almost reaches the ideal value 1/3. In addition, the final fidelity on the singlet state is as high as 95% with only these two multilevel oscillations. This experimentally operational optimization procedure shows comparable results to the previous optimization based on the number of occupied levels $K$, as shown in Fig. 6.

## VI. SCALING OF THE AMO TIME

The total AMO evolution time changes in general with the number of atoms in the spin-1 BEC. For each multilevel oscillation, we may estimate the evolution time by a half period of the Rabi oscillation between the ground and the first excited states. For the effective two-level model, the oscillating frequency is $f = \sqrt{\Omega^2 + \Delta^2}$, where $\Omega = q\langle 0|a_0^\dagger a_0|2\rangle = 2q\sqrt{N(N+3)}/(3\sqrt{5})$ is the coupling strength and $\Delta = 6c_2'/N$ the detuning. The effective half-period becomes $T_{mo}(q) = 0.5/f \approx 0.5/\sqrt{(6c_2'/N)^2 + (0.3qN)^2}$. The total AMO time is $T = T_a + \sum_i T_{mo}(q_i)$.

For the last multilevel oscillation, the coupling and the detuning are in the same order, $\Omega \sim \Delta$, so the half period is $T_{mo} \approx 0.5/(\sqrt{2}\,\Delta) \propto N$. For other multilevel oscillations, the coupling is much larger than the detuning of the ground and the first excited states. Thus the half period is $T_{mo} \approx 0.5/\Omega \propto 1/N$. Clearly, for large enough $N$, the AMO time scales as $N$. For the example presented in Fig. 3(a) in the main text, we find $T = 5.8$ s where $T_a = 0.9$ s, $T_{mo}(q_1) = 0.05$ s, $T_{mo}(q_2) = 1.73$ s, and $T_{mo}(q_3) = 3.12$ s. This estimation is in the same order as the numerical result. The total AMO time is dominated by the last multilevel oscillation. Compared to the adiabatic evolution whose time scales as $N^3$, the multilevel oscillation time is only $\sim 10^{-6}$ of it for $N = 1,000$.


[1] M. Scully and M. Zubairy, *Quantum Optics* (Cambridge University Press, Cambridge, England, 1997).
[2] D. M. Stamper-Kurn, M. R. Andrews, A. P. Chikkatur, S. Inouye, H.-J. Miesner, J. Stenger, and W. Ketterle, Phys. Rev. Lett. **80**, 2027 (1998).
[3] J. Stenger, S. Inouye, D. M. Stamperkurn, H. J. Miesner, A. P. Chikkatur, and W. Ketterle, Nature(London) **396**, 345 (1998).
[4] T.-L. Ho, Phys. Rev. Lett. **81**, 742 (1998).
[5] C. K. Law, H. Pu, and N. P. Bigelow, Phys. Rev. Lett. **81**, 5257 (1998).
[6] T. Ohmi and K. Machida, J. Phys. Soc. Jpn. **67**, 1822 (1998).
[7] L. Zhao, J. Jiang, T. Tang, M. Webb, and Y. Liu, Phys. Rev. A **89**, 023608 (2014).
[8] F. Gerbier, A. Widera, S. Fölling, O. Mandel, and I. Bloch, Phys. Rev. A **73**, 041602(R) (2006).
[9] S. R. Leslie, J. Guzman, M. Vengalattore, J. D. Sau, M. L. Cohen, and D. M. Stamper-Kurn, Phys. Rev. A **79**, 043631 (2009).
[10] H. Pu, C. K. Law, S. Raghavan, J. H. Eberly, and N. P. Bigelow, Phys. Rev. A **60**, 1463 (1999).
[11] S. Yi, O. E. Müstecaplıoğlu, C. P. Sun, and L. You, Phys. Rev. A **66**, 011601(R) (2002).
[12] Z. Zhang and L.-M. Duan, Phys. Rev. Lett. **111**, 180401 (2013).
[13] X.-Y. Luo, Y.-Q. Zou, L.-N. Wu, Q. Liu, M.-F. Han, M. K. Tey, and L. You, Science **355**, 620 (2017).
[14] L. D. Sarlo, L. Shao, V. Corre, T. Zibold, D. Jacob, J. Dalibard, and F. Gerbier, New J. Phys. **15**, 113039 (2013).
[15] B. W. Shore, *Manipulating Quantum Structure Using Laser Pulses* (Cambridge University Press, Cambridge, England, 2011).
[16] W. Zhang, D. L. Zhou, M.-S. Chang, M. S. Chapman, and L. You, Phys. Rev. A **72**, 013602 (2005).

[17] H. Li, Z. Pu, M. S. Chapman, and W. Zhang, Phys. Rev. A **92**, 013630 (2015).

[18] L. Chang, Q. Zhai, R. Lu, and L. You, Phys. Rev. Lett. **99**, 080402 (2007).
